# Supplementary material for: LAS-AT: Adversarial Training with Learnable Attack Strategy
Source: arXiv:2203.06616 source file (2022-03-13)
Supplement: Supplementary file 1 [file supplementary.tex]

\section*{Detailed Proof}

First we introduce some notations. Let $\mathcal{L}_0:\mathcal{X}\times\mathcal{Y}\times\mathcal{W}\times\boldsymbol{\Theta}\rightarrow\mathbb{R}^+$ be the objective function in \eqref{eq:newAT_pro} as
\begin{equation}
    \mathcal{L}_0 = \mathcal{L}_1+\alpha \mathcal{L}_2+\beta \mathcal{L}_3.
\end{equation}
We define $\boldsymbol{x}^*_{\text{adv}}(\boldsymbol{x},\mathbf{w})$ as the optimal adversarial example generated by the strategy network
\begin{equation}
    \begin{aligned}
        & \boldsymbol{x}^*_{\text{adv}}(\boldsymbol{x},\mathbf{w}) &=&\ \  \underset{\boldsymbol{\theta}}{\arg\max}\ g(\boldsymbol{x},\boldsymbol{a}(\boldsymbol{\theta}),\mathbf{w})\\
        & &=&\ \ \underset{\boldsymbol{\theta}}{\arg\max}\ \mathbb{E}_{\boldsymbol{a}\sim p(\boldsymbol{a}|\boldsymbol{x},\boldsymbol{\theta})}[\mathcal{L}_0],
    \end{aligned}
\end{equation}
and $\boldsymbol{\hat{x}}_{\text{adv}}(\boldsymbol{x},\mathbf{w})$ is a $\delta$-approximate solution to $\boldsymbol{x}^*_{\text{adv}}(\boldsymbol{x},\mathbf{w})$. In addition, the full gradient of $\mathcal{L}_0$ w.r.t $\mathbf{w}$ is 
\begin{equation}
    \label{eq:grad_1}
    \begin{aligned}
        & \nabla_{\mathbf{w}} \mathcal{L}_0(\mathbf{w}) &=&\ \  \frac{1}{N} \sum_{i=n}^N \nabla_{\mathbf{w}} \mathcal{L}^n_0\\
        & &=&\ \ \frac{1}{N} \sum_{n=1}^N \nabla_{\mathbf{w}} \mathcal{L}_0(\boldsymbol{x}^*_{\text{adv}}(\boldsymbol{x}_n,\mathbf{w}),\mathbf{w}),
    \end{aligned}
\end{equation}
where $\boldsymbol{x}^*_{\text{adv}}(\boldsymbol{x}_n)$ is the optimal adversarial example for $\boldsymbol{x}_n$. The stochastic gradient of $\mathcal{L}_0$ w.r.t $\mathbf{w}$ is 
\begin{equation}
 \label{eq:grad_2}
    \begin{aligned}
        & \nabla_{\mathbf{w}}\ell(\mathbf{w}) &=&\ \  \frac{1}{|\mathcal{B}|}\sum_{i=1}^{|\mathcal{B}|} \nabla_{\mathbf{w}} \mathcal{L}^i_0\\
        & &=&\ \ \frac{1}{|\mathcal{B}|} \sum_{n=1}^N \nabla_{\mathbf{w}} \mathcal{L}_0(\boldsymbol{x}^*_{\text{adv}}(\boldsymbol{x}_i,\mathbf{w}),\mathbf{w}).
    \end{aligned}
\end{equation}
Then $\nabla_{\boldsymbol{\theta}} \mathcal{L}_0$ and $\nabla_{\boldsymbol{\theta}}\ell$ correspond to the full and stochastic gradients of $\mathcal{L}_0$ w.r.t $\boldsymbol{\theta}$. Without lose of generality, we assume that
\begin{equation}
    \mathbb{E}[\nabla_{\mathbf{w}} \ell(\mathbf{w})] = \nabla_{\mathbf{w}}\mathcal{L}_0(\mathbf{w}).
\end{equation}
We note the approximate stochastic gradient as $\nabla_{\mathbf{w}}\hat{\ell}$:
\begin{equation}
     \label{eq:grad_3}
    \begin{aligned}
        & \nabla_{\mathbf{w}}\hat{\ell}~(\mathbf{w}) &=&\ \  \frac{1}{|\mathcal{B}|}\sum_{i=1}^{|\mathcal{B}|} \nabla_{\mathbf{w}} \hat{\mathcal{L}}^i_0\\
        & &=&\ \ \frac{1}{|\mathcal{B}|} \sum_{n=1}^N \nabla_{\mathbf{w}} \mathcal{L}_0(\hat{\boldsymbol{x}}_{\text{adv}}(\boldsymbol{x}_i,\mathbf{w}),\mathbf{w}).
    \end{aligned}    
\end{equation}
Moreover, the adversarial example $\boldsymbol{x}_{\text{adv}}(\boldsymbol{x},\mathbf{w})$ can be identified by a parameter $\boldsymbol{\theta}$ of the strategy network and the gradients like \eqref{eq:grad_1}, \eqref{eq:grad_2}, \eqref{eq:grad_3} would be
\begin{equation}
    \begin{aligned}
        & \nabla_{\mathbf{w}} \mathcal{L}_0(\boldsymbol{\theta},\mathbf{w}) &:=&\ \ \nabla_{\mathbf{w}} \mathcal{L}_0(\mathbf{w})\\
        & \nabla_{\mathbf{w}}\ell(\boldsymbol{\theta},\mathbf{w}) &:=&\ \ \nabla_{\mathbf{w}}\ell(\mathbf{w})\\
        & \nabla_{\mathbf{w}}\hat{\ell}(\boldsymbol{\theta},\mathbf{w}) &:=&\ \ \nabla_{\mathbf{w}}\hat{\ell}~(\mathbf{w}).
    \end{aligned}
\end{equation}
The corresponding gradients w.r.t $\boldsymbol{\theta}$ will be $\nabla_{\boldsymbol{\theta}} \mathcal{L}_0$, $\nabla_{\boldsymbol{\theta}} \ell$ and $\nabla_{\boldsymbol{\theta}} \hat{\ell}$. As the $\mathcal{L}_0$ in \eqref{eq:newAT_pro} satisfies the Lipschitz gradient conditions, given $\boldsymbol{x}_n\in\mathcal{X}$, it holds that
\begin{equation}
    \label{eq:lipschitz_grad}
    \begin{aligned}
        & &&\ \ \underset{\boldsymbol{\theta}}{\sup}\ \|\nabla_{\mathbf{w}} \mathcal{L}^n_0(\boldsymbol{\theta},\mathbf{w})-\nabla_{\mathbf{w}} \mathcal{L}^n_0(\boldsymbol{\theta},\mathbf{w}')\|_2\\
        & &\leq&\ \  L_{\mathbf{w}\mathbf{w}}\|\mathbf{w}-\mathbf{w}'\|_2\\[5pt]
        & & &\ \ \underset{\mathbf{w}}{\sup}\ \|\nabla_{\mathbf{w}} \mathcal{L}^n_0(\boldsymbol{\theta},\mathbf{w})-\nabla_{\mathbf{w}} \mathcal{L}^n_0(\boldsymbol{\theta}',\mathbf{w})\|_2\\
        & &\leq&\ \ L_{\mathbf{w}\boldsymbol{\theta}}\|\boldsymbol{\theta}-\boldsymbol{\theta}'\|_2\\[5pt]
        & & &\ \ \underset{\boldsymbol{\theta}}{\sup}\ \|\nabla_{\boldsymbol{\theta}} \mathcal{L}^n_0(\boldsymbol{\theta},\mathbf{w})-\nabla_{\boldsymbol{\theta}} \mathcal{L}^n_0(\boldsymbol{\theta},\mathbf{w}')\|_2\\
        & &\leq&\ \  L_{\boldsymbol{\theta}\mathbf{w}}\|\mathbf{w}-\mathbf{w}'\|_2,
    \end{aligned}
\end{equation}
where $L_{\mathbf{w}\mathbf{w}}$, $L_{\mathbf{w}\boldsymbol{\theta}}$ and $L_{\boldsymbol{\theta}\mathbf{w}}$ are positive constants. Furthermore, by the strongly-concavity of $\mathcal{L}_0$ and given $\boldsymbol{x}_n\in\mathcal{X}$, we know that for any $\boldsymbol{\theta}_1$ and $\boldsymbol{\theta}_2\in\boldsymbol{\Theta}$,
\begin{equation}
    \begin{aligned}
        & &&\ \ \mathcal{L}^n_0(\boldsymbol{\theta}_1,\mathbf{w})-\mathcal{L}^n_0( \boldsymbol{\theta}_2,\mathbf{w})\\[5pt]
        & &\leq&\ \ \big\langle\nabla_{\boldsymbol{\theta}} \mathcal{L}^n_0(\boldsymbol{\theta},\mathbf{w}),\boldsymbol{\theta}_1-\boldsymbol{\theta}_2\big\rangle - \frac{\mu}{2}\|\boldsymbol{\theta}_1-\boldsymbol{\theta}_2\|_2^2.
    \end{aligned}
\end{equation}
As the variance of the stochastic gradient is bounded by $\sigma^2>0$, it means that
\begin{equation}
    \mathbb{E}\big[\|\nabla_{\mathbf{w}} \ell(\mathbf{w})-\nabla_{\mathbf{w}} \mathcal{L}_0(\mathbf{w})\|^2_2\big]\leq\sigma^2.
\end{equation}

To prove the main result, we need the following two important lemmas.
\begin{lemma}
\label{lem:1}
Suppose that $\mathcal{L}_0$ in \eqref{eq:newAT_pro} satisfies the Lipschitz gradient conditions as \eqref{eq:lipschitz_grad} and $\mathcal{L}_0$ is $\mu$-strongly concave in $\boldsymbol{\Theta}$, we have $\mathcal{L}_0$ is Lipschitz smooth with $L_0$ 
\begin{equation}
    L_0=\frac{L_{\mathbf{w}\boldsymbol{\theta}}L_{\boldsymbol{\theta}\mathbf{w}}}{\mu}+L_{\mathbf{w}\mathbf{w}}.
\end{equation}
It holds that
\begin{equation}
    \begin{aligned}
    & \mathcal{L}_0(\mathbf{w}_1)\leq\mathcal{L}_0(\mathbf{w}_2)&+&\ \ \ \left\langle\nabla_{\mathbf{w}} \mathcal{L}_0(\mathbf{w}_2),\mathbf{w}_1-\mathbf{w}_2\right\rangle\\
    & &+&\ \ \ \frac{L_0}{2}\|\mathbf{w}_1-\mathbf{w}_2\|^2_2,
    \end{aligned}
\end{equation}
and
\begin{equation}
    \left\|\nabla_{\mathbf{w}} \mathcal{L}_0-\nabla_{\mathbf{w}} \mathcal{L}_0(\mathbf{w}_2)\right\|_2\leq L_0\|\mathbf{w}_1-\mathbf{w}_2\|_2.
\end{equation}
\end{lemma}
\begin{proof}
By the strongly-concavity of $\mathcal{L}_0$ and given $\boldsymbol{x}_n\in\mathcal{X}$, for any $\boldsymbol{\theta}_1$, $\boldsymbol{\theta}_2$ and the corresponding $\mathbf{w}_1$, $\mathbf{w}_2$ , we have
\begin{equation}
    \label{eq:30}
    \begin{aligned}
        & &&\ \ \mathcal{L}^n_0(\boldsymbol{\theta}_1,\mathbf{w}_2)-\mathcal{L}^n_0( \boldsymbol{\theta}_2,\mathbf{w}_2)\\[5pt]
        & &\leq&\ \ \big\langle\nabla_{\boldsymbol{\theta}} \mathcal{L}^n_0(\boldsymbol{\theta}_2,\mathbf{w}_2),\boldsymbol{\theta}_1-\boldsymbol{\theta}_2\big\rangle - \frac{\mu}{2}\|\boldsymbol{\theta}_1-\boldsymbol{\theta}_2\|_2^2\\[3pt]
        & &\leq&\ \ -\frac{\mu}{2}\|\boldsymbol{\theta}_1-\boldsymbol{\theta}_2\|_2^2.
    \end{aligned}    
\end{equation}
The second inequality is true as 
$$
    \langle\nabla_{\boldsymbol{\theta}} \mathcal{L}^n_0(\boldsymbol{\theta}_2,\mathbf{w}_2),\boldsymbol{\theta}_1-\boldsymbol{\theta}_2\rangle\leq 0.
$$
In addition, we have
\begin{equation}
    \label{eq:31}
    \begin{aligned}
        & &&\ \ \mathcal{L}^n_0(\boldsymbol{\theta}_2,\mathbf{w}_2)-\mathcal{L}^n_0( \boldsymbol{\theta}_1,\mathbf{w}_2)\\[5pt]
        & &\leq&\ \ \big\langle\nabla_{\boldsymbol{\theta}} \mathcal{L}^n_0(\boldsymbol{\theta}_1,\mathbf{w}_2),\boldsymbol{\theta}_2-\boldsymbol{\theta}_1\big\rangle - \frac{\mu}{2}\|\boldsymbol{\theta}_1-\boldsymbol{\theta}_2\|_2^2\\[3pt]
        & &\leq&\ \ -\frac{\mu}{2}\|\boldsymbol{\theta}_1-\boldsymbol{\theta}_2\|_2^2.
    \end{aligned}  
\end{equation}
Combining \eqref{eq:30} and \eqref{eq:31}, we have
\begin{equation}
    \label{eq:32}
    \begin{aligned}
        & & &\ \ \mu\|\boldsymbol{\theta}_1-\boldsymbol{\theta}_2\|^2_2\\[5pt]
        & &\leq&\ \ \langle\nabla_{\boldsymbol{\theta}} \mathcal{L}^n_0(\boldsymbol{\theta}_1,\mathbf{w}_2),\boldsymbol{\theta}_2-\boldsymbol{\theta}_1\rangle\\[5pt]
        & &\leq&\ \ \langle\nabla_{\boldsymbol{\theta}} \mathcal{L}^n_0(\boldsymbol{\theta}_1,\mathbf{w}_2)-\nabla_{\boldsymbol{\theta}} \mathcal{L}^n_0(\boldsymbol{\theta}_1,\mathbf{w}_1),\boldsymbol{\theta}_2-\boldsymbol{\theta}_1\rangle\\[5pt]
        & &\leq&\ \ \|\nabla_{\boldsymbol{\theta}} \mathcal{L}^n_0(\boldsymbol{\theta}_1,\mathbf{w}_2)-\nabla_{\boldsymbol{\theta}} \mathcal{L}^n_0(\boldsymbol{\theta}_1,\mathbf{w}_1)\|_2\|\boldsymbol{\theta}_2-\boldsymbol{\theta}_1\|_2\\[5pt]
        & &\leq&\ \ L_{\boldsymbol{\theta}\mathbf{w}}\|\mathbf{w}_2-\mathbf{w}_1\|_2\|\boldsymbol{\theta}_2-\boldsymbol{\theta}_1\|_2,
    \end{aligned}
\end{equation}
where the second inequality holds as
$$
    \langle\nabla_{\boldsymbol{\theta}} \mathcal{L}^n_0(\boldsymbol{\theta}_1,\mathbf{w}_1),\boldsymbol{\theta}_2-\boldsymbol{\theta}_1\rangle\leq 0,
$$
the third inequality follows from the Cauchy-Schwarz inequality, and the last one holds by the Lipschitz smoothness of the gradients of $\mathcal{L}_0$ \eqref{eq:lipschitz_grad}. 

For any $n\in[N]$, we have
\begin{equation}
    \begin{aligned}
       & & &\ \ \|\nabla_{\mathbf{w}} \mathcal{L}^n_0(\boldsymbol{\theta}_1,\mathbf{w}_1)-\nabla_{\mathbf{w}} \mathcal{L}^n_0(\boldsymbol{\theta}_2,\mathbf{w}_2)\|_2\\[5pt]
       & &\leq&\ \ \|\nabla_{\mathbf{w}} \mathcal{L}^n_0(\boldsymbol{\theta}_1,\mathbf{w}_1)-\nabla_{\mathbf{w}} \mathcal{L}^n_0(\boldsymbol{\theta}_2,\mathbf{w}_1)\|_2\\[5pt]
       & & &\ \ +\|\nabla_{\mathbf{w}} \mathcal{L}^n_0(\boldsymbol{\theta}_2,\mathbf{w}_1)-\nabla_{\mathbf{w}} \mathcal{L}^n_0(\boldsymbol{\theta}_2,\mathbf{w}_2)\|_2\\[5pt]
       & &\leq&\ \ L_{\mathbf{w}\boldsymbol{\theta}}\|\boldsymbol{\theta}_1-\boldsymbol{\theta}_2\|_2+L_{\mathbf{w}\mathbf{w}}\|\mathbf{w}_1-\mathbf{w}_2\|_2\\[5pt]
       & &=&\ \ \left(\frac{L_{\mathbf{w}\boldsymbol{\theta}}L_{\boldsymbol{\theta}\mathbf{w}}}{\mu}+L_{\mathbf{w}\mathbf{w}}\right)\|\mathbf{w}_1-\mathbf{w}_2\|_2,
    \end{aligned}
\end{equation}
where the first inequality follows from the triangle inequality, and the second inequality holds due to \eqref{eq:32} and the Lipschitz smoothness of the gradients of $\mathcal{L}_0$ \eqref{eq:lipschitz_grad}. By the definition of $\mathcal{L}$, it holds that
\begin{equation}
    \begin{aligned}
        & & &\ \ \|\nabla_{\mathbf{w}} \mathcal{L}_0(\mathbf{w}_1)-\nabla_{\mathbf{w}} \mathcal{L}_0(\mathbf{w}_2)\|_2\\[5pt]
        & &=&\ \ \left\|\frac{1}{N}\sum_{n=1}^N \left(\nabla_{\mathbf{w}} \mathcal{L}^n_0(\boldsymbol{\theta}_1,\mathbf{w}_1)-\nabla_{\mathbf{w}} \mathcal{L}^n_0(\boldsymbol{\theta}_2,\mathbf{w}_2)\right)\right\|_2\\
        & &\leq&\ \ \frac{1}{N}\sum_{n=1}^N\|\nabla_{\mathbf{w}} \mathcal{L}^n_0(\boldsymbol{\theta}_1,\mathbf{w}_1)-\nabla_{\mathbf{w}} \mathcal{L}^n_0(\boldsymbol{\theta}_2,\mathbf{w}_2)\|_2\\
        & &\leq&\ \ \left(\frac{L_{\mathbf{w}\boldsymbol{\theta}}L_{\boldsymbol{\theta}\mathbf{w}}}{\mu}+L_{\mathbf{w}\mathbf{w}}\right)\|\mathbf{w}_1-\mathbf{w}_2\|_2.
    \end{aligned}
\end{equation}
With the definition of the Lipschitz smoothness, we complete the proof.
\end{proof}

\begin{lemma}
\label{lem:2}
Suppose that $\mathcal{L}_0$ in \eqref{eq:newAT_pro} satisfies the Lipschitz gradient conditions as \eqref{eq:lipschitz_grad} and $\mathcal{L}_0$ is $\mu$-strongly concave in $\boldsymbol{\Theta}$, the approximate stochastic gradient $\nabla_{\mathbf{w}}\hat{\ell}(\mathbf{w})$ \eqref{eq:grad_3} satisfies
\begin{equation}
    \|\nabla_{\mathbf{w}}\hat{\ell}~(\mathbf{w})-\nabla_{\mathbf{w}}\ell(\mathbf{w})\|_2\leq L_{\mathbf{w}\boldsymbol{\theta}}\sqrt{\frac{\delta}{\mu}},
\end{equation}
where $\boldsymbol{\hat{x}}_{\text{adv}}(\boldsymbol{x},\mathbf{w})$ is a $\delta$-approximate solution to $\boldsymbol{x}^*_{\text{adv}}(\boldsymbol{x},\mathbf{w})$ with given $\boldsymbol{x}\in\mathcal{X}$.
\end{lemma}
\begin{proof}
By the definitions of $\nabla_{\mathbf{w}}\hat{\ell}$ and $\nabla_{\mathbf{w}}\ell$, we have
\begin{equation}
    \label{eq:36}
    \begin{aligned}
    & &&\ \ \|\nabla_{\mathbf{w}}\hat{\ell}~(\mathbf{w})-\nabla_{\mathbf{w}}\ell(\mathbf{w})\|_2\\[5pt]
    & &=&\ \ \left\|\frac{1}{|\mathcal{B}|} \sum_{i=1}^{|\mathcal{B}|} (\nabla_{\mathbf{w}} \mathcal{L}_0(\boldsymbol{\hat{x}}_{\text{adv}}(\boldsymbol{x}_i,\mathbf{w}),\mathbf{w})\right.\\
    & & &\ \ \left.\textcolor{white}{\frac{1}{|\mathcal{B}|} \sum_{i=1}^{|\mathcal{B}|}}-\nabla_{\mathbf{w}}\mathcal{L}_0(\boldsymbol{x}^*_{\text{adv}}(\boldsymbol{x}_i,\mathbf{w}),\mathbf{w}))\right\|_2\\
    & &\leq&\ \ \frac{1}{|\mathcal{B}|} \sum_{n=1}^N \left\|\nabla_{\mathbf{w}} \mathcal{L}_0(\boldsymbol{\hat{x}}_{\text{adv}}(\boldsymbol{x}_i,\mathbf{w}),\mathbf{w})\right.\\
    & & &\ \ \textcolor{white}{\frac{1}{|\mathcal{B}|} \sum_{i=1}^{|\mathcal{B}|}}\left.-\nabla_{\mathbf{w}}\mathcal{L}_0(\boldsymbol{x}^*_{\text{adv}}(\boldsymbol{x}_i,\mathbf{w}),\mathbf{w})\right\|_2\\[5pt]
    & &\leq&\ \ \frac{1}{|\mathcal{B}|} \sum_{i=1}^{|\mathcal{B}|} L_{\mathbf{w}\boldsymbol{\theta}}\|\boldsymbol{\hat{\theta}}-\boldsymbol{\theta}^*\|_2,
    \end{aligned}
\end{equation}
where the second inequality follows from the triangle inequality, the third inequality holds due to the gradient Lipschitz condition, and $\boldsymbol{\hat{\theta}}$ is the parameter of strategy network corresponding to $\boldsymbol{\hat{x}}_{\text{adv}}(\boldsymbol{x}_i,\mathbf{w})$, $\boldsymbol{\theta}^*$ is similar.

Since $\boldsymbol{\hat{x}}_{\text{adv}}(\boldsymbol{x}_i,\mathbf{w})$ is a $\delta$-approximate adversarial example generated by the strategy network, we have
\begin{equation}
    \label{eq:37}
    \left\langle\boldsymbol{\theta}^*-\boldsymbol{\hat{\theta}}, \nabla_{\boldsymbol{\theta}} \mathcal{L}_0(\boldsymbol{\hat{\theta}},\mathbf{w})\right\rangle\leq \delta.
\end{equation}
In addition, it holds that
\begin{equation}
    \label{eq:38}
    \left\langle\boldsymbol{\hat{\theta}}-\boldsymbol{\theta}^*, \nabla_{\boldsymbol{\theta}} \mathcal{L}_0(\boldsymbol{\theta}^*,\mathbf{w})\right\rangle\leq 0.
\end{equation}
Putting \eqref{eq:37} and \eqref{eq:38} together gives birth to
\begin{equation}
    \label{eq:39}
    \left\langle\boldsymbol{\hat{\theta}}-\boldsymbol{\theta}^*,\nabla_{\boldsymbol{\theta}} \mathcal{L}_0(\boldsymbol{\theta}^*,\mathbf{w})-\nabla_{\boldsymbol{\theta}} \mathcal{L}_0(\boldsymbol{\hat{\theta}},\mathbf{w})\right\rangle\leq \delta.
\end{equation}
Moreover, by the strongly concavity of $\mathcal{L}_0$ and \eqref{eq:32}, we have
\begin{equation}
    \label{eq:40}
    \begin{aligned}
        & & &\ \ \mu\|\boldsymbol{\theta}^*-\boldsymbol{\hat{\theta}}\|^2_2\\[2.5pt]
        & &\leq&\ \ \langle\nabla_{\boldsymbol{\theta}}\mathcal{L}^n_0(\boldsymbol{\theta}^*,\mathbf{w})-\nabla_{\boldsymbol{\theta}} \mathcal{L}^n_0(\boldsymbol{\hat{\theta}},\mathbf{w}),\boldsymbol{\hat{\theta}}-\boldsymbol{\theta}^*\rangle\\[5pt]
        & &\leq&\ \ \delta.
    \end{aligned}
\end{equation}
Consequently, it immediately yields
\begin{equation}
    \label{eq:41}
    \|\boldsymbol{\theta}^*-\boldsymbol{\hat{\theta}}\|_2\leq\sqrt{\frac{\delta}{\mu}}.
\end{equation}
Substituting \eqref{eq:41} into \eqref{eq:36}, we complete the proof.
\end{proof}

\convergence*
\begin{proof}
% Let 
% \begin{equation}
%     \begin{aligned}
%         & \mathcal{\bar{L}}^*(\mathbf{w}) &=&\ \  \frac{1}{N}\sum_{n=1}^{N}\underset{\boldsymbol{x}_{\text{adv}}}{\max}~\mathcal{L}_0(\boldsymbol{x}_{\text{adv}}(\boldsymbol{x}_n,\mathbf{w}),\mathbf{w})\\[5pt]
%         & &=&\ \ \frac{1}{N}\sum_{n=1}^{N}~\mathcal{L}_0(\boldsymbol{x}^*_{\text{adv}}(\boldsymbol{x}_n,\mathbf{w}),\mathbf{w}).
%     \end{aligned}
% \end{equation}
By Lemma \ref{lem:1}, we have
\begin{equation*}
    \begin{aligned}
        & \mathcal{L}_0(\mathbf{w}^{t+1})&\leq&\ \ \mathcal{L}_0(\mathbf{w}^t)+\frac{L_0}{2}\|\mathbf{w}^{t+1}-\mathbf{w}^{t}\|^2_2\\[5pt]
        & &+&\ \ \left\langle\nabla_{\mathbf{w}} \mathcal{L}_0(\mathbf{w}^t),\mathbf{w}^{t+1}-\mathbf{w}^{t}\right\rangle.
    \end{aligned}    
\end{equation*}
Due to
\[
    \mathbf{w}^{t+1}=\mathbf{w}^{t}-\eta_t\nabla_{\mathbf{w}}\hat{\ell}(\mathbf{w}^{t}),
\]
it holds that
\begin{equation}
    \begin{aligned}
        & & &\ \ \mathcal{L}_0(\mathbf{w}^{t+1})\\[5pt]
        & &\leq&\ \ \mathcal{L}_0(\mathbf{w}^t)-\eta_t\|\nabla_{\mathbf{w}}\mathcal{L}_0(\mathbf{w}^t)\|_2^2+\frac{L_0\eta_t^2}{2}\|\nabla_{\mathbf{w}}\hat{\ell}(\mathbf{w}^{t})\|_2^2\\[5pt]
        & & &\ \ +\eta_t\langle\nabla_{\mathbf{w}}\mathcal{L}_0(\mathbf{w}^t),\nabla_{\mathbf{w}}\mathcal{L}_0(\mathbf{w}^t)-\nabla_{\mathbf{w}}\hat{\ell}(\mathbf{w}^{t})\rangle\\[5pt]
        & &=&\ \ \mathcal{L}_0(\mathbf{w}^t)-\eta_t\left(1-\frac{L_0\eta_t}{2}\right)\|\nabla_{\mathbf{w}}\mathcal{L}_0(\mathbf{w}^t)\|_2^2\\[5pt]
        & & &\ \ +\eta_t\left(1-\frac{L_0\eta_t}{2}\right)\langle\nabla_{\mathbf{w}}\mathcal{L}_0(\mathbf{w}^t),\nabla_{\mathbf{w}}\mathcal{L}_0(\mathbf{w}^t)-\nabla_{\mathbf{w}}\hat{\ell}(\mathbf{w}^{t})\rangle\\[5pt]
        & & &\ \ + \frac{L_0\eta_t^2}{2}\|\nabla_{\mathbf{w}}\hat{\ell}(\mathbf{w}^{t})-\nabla_{\mathbf{w}}\mathcal{L}_0(\mathbf{w}^t)\|_2^2\\[5pt]
        & &=&\ \ \mathcal{L}_0(\mathbf{w}^t)-\eta_t\left(1-\frac{L_0\eta_t}{2}\right)\|\nabla_{\mathbf{w}}\mathcal{L}_0(\mathbf{w}^t)\|_2^2\\[5pt]
        & & &\ \ +\eta_t\left(1-\frac{L_0\eta_t}{2}\right)\langle\nabla_{\mathbf{w}}\mathcal{L}_0(\mathbf{w}^t),\nabla_{\mathbf{w}}\ell(\mathbf{w}^{t})-\nabla_{\mathbf{w}}\hat{\ell}(\mathbf{w}^{t})\rangle\\[5pt]
        & & &\ \ +\eta_t\left(1-\frac{L_0\eta_t}{2}\right)\langle\nabla_{\mathbf{w}}\mathcal{L}_0(\mathbf{w}^t),\nabla_{\mathbf{w}}\mathcal{L}_0(\mathbf{w}^t)-\nabla_{\mathbf{w}}\ell(\mathbf{w}^{t})\rangle\\[5pt]
        & & &\ \ +\frac{L_0\eta_t^2}{2}\|\nabla_{\mathbf{w}}\hat{\ell}(\mathbf{w}^{t})-\nabla_{\mathbf{w}}\ell(\mathbf{w}^{t})+\nabla_{\mathbf{w}}\ell(\mathbf{w}^{t})-\nabla_{\mathbf{w}}\mathcal{L}_0(\mathbf{w}^t)\|_2^2\\
        & &\leq&\ \ \mathcal{L}_0(\mathbf{w}^t)-\frac{\eta_t}{2}\left(1-\frac{L_0\eta_t}{2}\right)\|\nabla_{\mathbf{w}}\mathcal{L}_0(\mathbf{w}^t)\|_2^2\\[5pt]
        & & &\ \ +\frac{\eta_t}{2}\left(1-\frac{L_0\eta_t}{2}\right)\|\nabla_{\mathbf{w}}\ell(\mathbf{w}^{t})-\nabla_{\mathbf{w}}\hat{\ell}(\mathbf{w}^{t})\|^2_2\\[5pt]
        & & &\ \ +\eta_t\left(1+\frac{L_0\eta_t}{2}\right)\langle\nabla_{\mathbf{w}}\mathcal{L}_0(\mathbf{w}^t),\nabla_{\mathbf{w}}\mathcal{L}_0(\mathbf{w}^t)-\nabla_{\mathbf{w}}\ell(\mathbf{w}^{t})\rangle\\[5pt]
        & & &\ \ +L_0\eta_t^2\|\nabla_{\mathbf{w}}\hat{\ell}(\mathbf{w}^{t})-\nabla_{\mathbf{w}}\ell(\mathbf{w}^{t})\|_2^2\\[5pt]
        & & &\ \ +L_0\eta_t^2\|\nabla_{\mathbf{w}}\ell(\mathbf{w}^{t})-\nabla_{\mathbf{w}}\mathcal{L}_0(\mathbf{w}^t)\|_2^2\\
    \end{aligned}
\end{equation}
Taking expectation on both sides of the above inequality conditioned on $\mathbf{w}^t$, then we have
\begin{equation}
    \begin{aligned}
        & & &\ \ \mathbb{E}[\mathcal{L}_0(\mathbf{w}^{t+1})-\mathcal{L}_0(\mathbf{w}^{t})|\mathbf{w}^t]\\[5pt]
        & &\leq&\ \ -\frac{\eta_t}{2}\left(1-\frac{L_0\eta_t}{2}\right)\|\nabla_{\mathbf{w}}\mathcal{L}_0(\mathbf{w}^t)\|_2^2\\[5pt]
        & & &\ \ +\frac{\eta}{2}\left(1+\frac{3\eta_tL_0}{2}\right)\frac{\delta L^2_{\mathbf{w}\boldsymbol{\theta}}}{\mu}+L_0\eta^2_t\sigma^2.
    \end{aligned}
\end{equation}
Then we do the telescope sum over $t=0,\dots,T-1$, we obtain
\begin{equation}
    \begin{aligned}
        & & &\ \ \sum_{t=0}^{T-1}\frac{\eta_t}{2}\left(1-\frac{L_0\eta_t}{2}\right)\mathbb{E}[\|\mathcal{L}_0(\mathbf{w}^{t})\|^2_2]\\[5pt]
        & &\leq&\ \ \mathbb{E}[\mathcal{L}_0(\mathbf{w}^0)-\mathcal{L}_0(\mathbf{w}^T)]+L_0\sum_{t=0}^{T-1}\eta^2_t\sigma^2\\[5pt]
        & & &\ \ + \sum_{t=0}^{T-1}\frac{\eta}{2}\left(1+\frac{3\eta_tL_0}{2}\right)\frac{\delta L^2_{\mathbf{w}\boldsymbol{\theta}}}{\mu}.
    \end{aligned}
\end{equation}
Choosing $\eta_t= \eta_1$ as
\begin{equation}
    \eta_1 = \min\left(\frac{1}{L_0},\ \sqrt{\frac{\mathcal{L}_0(\mathbf{w}^0)-\underset{\mathbf{w}}{\min}\ \mathcal{L}_0(\mathbf{w})}{\sigma^2TL_0}}\right),
\end{equation}
it holds that
\begin{equation}
    \frac{1}{T}\sum_{t=0}^{T-1}\mathbb{E}\big[\|\nabla \mathcal{L}_0(\mathbf{w}^t)\|^2_2\big]\leq4\sigma\sqrt{\frac{\Delta L_0}{T}}+\frac{5\delta L^2_{\mathbf{w}\boldsymbol{\theta}}}{\mu},
\end{equation}
where $\Delta=\mathcal{L}_0(\mathbf{w}^0)-\underset{\mathbf{w}}{\min}\ \mathcal{L}_0(\mathbf{w})$.
\end{proof}
